# Supplementary material for: Adaptive Neural Compilation
Source: arXiv:1605.07969 source file (2016-05-26)
Supplement: Supplementary file 1 [file supplementary.tex]

\documentclass{article}
\PassOptionsToPackage{sort,square,comma,numbers}{natbib}
% if you need to pass options to natbib, use, e.g.:
% \PassOptionsToPackage{numbers, compress}{natbib}
% before loading nips_2016
%
% to avoid loading the natbib package, add option nonatbib:
% \usepackage[nonatbib]{nips_2016}

% to compile a camera-ready version, add the [final] option, e.g.:
\usepackage[final]{nips_2016}

\usepackage[utf8]{inputenc} % allow utf-8 input
\usepackage[T1]{fontenc}    % use 8-bit T1 fonts
\usepackage{hyperref}       % hyperlinks
\usepackage{url}            % simple URL typesetting
\usepackage{booktabs}       % professional-quality tables
\usepackage{amsfonts}       % blackboard math symbols
\usepackage{nicefrac}       % compact symbols for 1/2, etc.
\usepackage{microtype}      % microtypography

% My own includes
\usepackage{amsmath}
\usepackage{mathtools}
\usepackage{subcaption}
\usepackage{tikz}
\usepackage{placeins}
\usepackage{bbm}
\usepackage{bm}
\usepackage{listings}
\usepackage[lighttt]{lmodern}
\usepackage{framed}

\title{%
    Adaptive Neural Compilation \\
    \vspace{7pt}
    \large Supplementary Materials}

% The \author macro works with any number of authors. There are two
% commands used to separate the names and addresses of multiple
% authors: \And and \AND.
% 
% Using \And between authors leaves it to LaTeX to determine where to
% break the lines. Using \AND forces a line break at that point. So,
% if LaTeX puts 3 of 4 authors names on the first line, and the last
% on the second line, try using \AND instead of \And before the third
% author name.

\lstdefinelanguage{neulang}
{
  % list of keywords
  morekeywords=[2]{STOP,ZERO,INC,ADD,SUB,DEC,MIN,MAX,READ,WRITE,JEZ},
  morekeywords=[3]{var},
  sensitive=true, % keywords are not case-sensitive
}

\lstset{
  language={neulang},
  basicstyle=\normalfont\ttfamily, % Global Code Style
  keywordstyle=\normalfont\ttfamily,
  keywordstyle=[2]\bfseries,
  keywordstyle=[3]\bfseries,
  captionpos=b, % Position of the Caption (t for top, b for bottom)
  extendedchars=true, % Allows 256 instead of 128 ASCII characters
  tabsize=2, % number of spaces indented when discovering a tab
  columns=fixed, % make all characters equal width
  frame=trbl, % draw a frame at the top, right, left and bottom of the listing
  frameround=tttt, % make the frame round at all four corners
  framesep=4pt, % quarter circle size of the round corners
  numbers=left, % show line numbers at the left
  numberstyle=\tiny\ttfamily, % style of the line numbers
}

\begin{document}

\maketitle

\input{supplementary-content.tex}

\bibliographystyle{plainnat}
\bibliography{bibliography}

\end{document}
